# Supplementary material for: What is Missing? Explaining Neurons Activated by Absent Concepts
Source: arXiv:2603.09787 source file (2026-05-29)
Supplement: Supplementary file 1 [file mechanistic_bias.tex]

\begin{tikzpicture}[x=2cm,y=1.6cm]%
\sffamily
\scriptsize

;
\def\xTwo{0.8};
\def\xThree{1.6};

\colorlet{myred}{red!80!black}
\colorlet{myblue}{blue!80!black}
\colorlet{mygreen}{green!60!black}
\colorlet{mygray}{gray!60!black}

\colorlet{myorange}{orange!70!red!60!black}
\colorlet{mydarkred}{red!30!black}
\colorlet{mydarkblue}{blue!40!black}
\colorlet{mydarkgreen}{green!30!black}

\tikzstyle{blockOne} = [draw, color=colorSchemeOne, text centered, rectangle,
minimum height=0.51cm,minimum width=0.51cm, align=center]

\tikzstyle{blockTwo} = [draw, color=colorSchemeTwo, text centered, rectangle,
minimum height=0.51cm,minimum width=0.51cm, align=center]

\tikzset{
  >=latex, %
  node/.style={thick,circle,draw=mygray!30!black,minimum size=22,inner sep=0.5,outer sep=0.6},
  node in/.style={node,green!20!black,draw=mygray!30!black,fill=black!15},
  node trans/.style={node,green!20!black,draw=mygray!30!black,fill=black!15, opacity=0},
  node hidden/.style={node,blue!20!black,draw=myblue!30!black,fill=myblue!20},
  node hidden_concept/.style={node,blue!20!black,draw=myblue!30!black,fill overzoom image=example-image},
  node hidden_concept_one_exclusive/.style={node,blue!20!black,draw=myblue!30!black,fill overzoom image=images/beak.jpg},
  node hidden_concept_beak/.style={node,blue!20!black,draw=myblue!30!black,fill overzoom image=images/beak.jpg},
  node hidden_concept_mirror/.style={node,blue!20!black,draw=myblue!30!black,fill overzoom image=images/mirror.jpg},
  node hidden_concept_superposition/.style={node,blue!20!black,draw=myblue!30!black,fill overzoom image=images/tail_wheel.jpg},
  node hidden_concept_tail/.style={node,blue!20!black,draw=myblue!30!black,fill overzoom image=images/tail.jpg},
  node hidden_concept_wheel/.style={node,blue!20!black,draw=myblue!30!black,fill overzoom image=images/wheel.jpg},
  node label1/.style={thick,minimum height=13,minimum width=32,inner sep=0.5,outer sep=0.9,rectangle,draw=colorConceptOne,label=center:Bird},
  node label2/.style={thick,minimum height=13,minimum width=32,inner sep=0.5,outer sep=0.9,rectangle,draw=colorConceptTwo,label=center:Car},
  node convol/.style={node,orange!20!black,draw=myorange!30!black,fill=myorange!20},
  node out/.style={node,red!20!black,draw=myred!30!black,fill=myred!20},
  connect/.style={black!70}, %
  connect arrow/.style={-{Latex[length=4,width=3.5]},mydarkblue,shorten <=0.5,shorten >=1},
  node 1/.style={node in}, %
  node 2/.style={node hidden},
  node 3/.style={node out}
}

\newcommand\barplot{} %
\def\barplot[#1](#2,#3)(#4:#5){%
  \draw[draw=none, fill=gray] (#2, #3) rectangle ++(0.075,#4);
  \draw[line width=0.005mm,color=gray] (#2-0.04,#3) -- (#2+0.075+0.04,#3);
  \draw[line width=0.005mm,color=gray] (#2-0.04,#3+0.3) -- (#2+0.075+0.04,#3+0.3);
  
}

\newcommand\irregularcircle[2]{%
  \pgfextra {\pgfmathsetmacro\len{(#1)+rand*(#2)}}
  +(0:\len pt)
  \foreach \a in {10,20,...,350}{
    \pgfextra {\pgfmathsetmacro\len{(#1)+rand*(#2)}}
    -- +(\a:\len pt)
  } -- cycle
}

\def\NO{3} %
\def\NL{1} %
\def\yshift{0.0} %

  \foreach \i [evaluate={\c=int(\i==\NO); \y=\NO/2-\i-\c*\yshift; \index=(\i<\NO?int(\i):"m");}]
    in {\NO,...,1}{ %

    \ifnum\i=1 %

      \node[node in] (NO-\i) at (\xTwo,\y) {};

      \coordinate (c) at (\xTwo-0.65,\y);
      \draw[thick, colorSchemeOne, fill=colorSchemeOne!20,rounded corners=0.05cm] (c) \irregularcircle{0.65cm}{0.05cm};
      \node (rect) [blockOne,xshift=0.0cm, yshift=-0.0cm] at (\xTwo-0.65,\y-0.15) {};
      \node[inner sep=0pt] (img) at (\xTwo-0.65,\y-0.15) {\includegraphics[width=0.5cm]{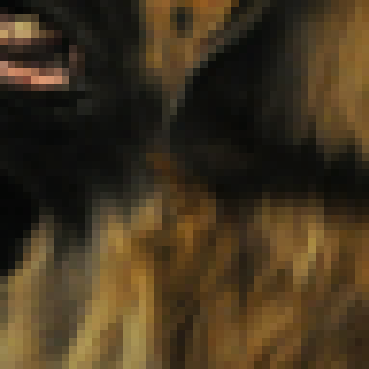}};
      \node (rect) [blockOne,xshift=0.0cm, yshift=-0.0cm] at (\xTwo-0.75,\y+0.1) {};
      \node[inner sep=0pt] (img) at (\xTwo-0.75,\y+0.1) {\includegraphics[width=0.5cm]{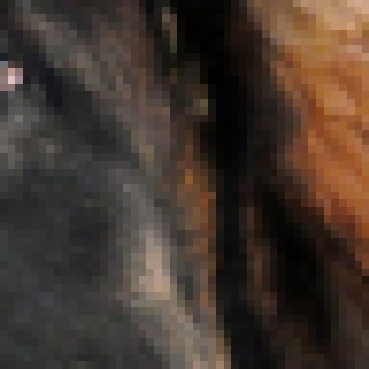}};
      \node (rect) [blockOne,xshift=0.0cm, yshift=-0.0cm] at (\xTwo-0.55,\y+0.08) {};
      \node[inner sep=0pt] (img) at (\xTwo-0.55,\y+0.08) {\includegraphics[width=0.5cm]{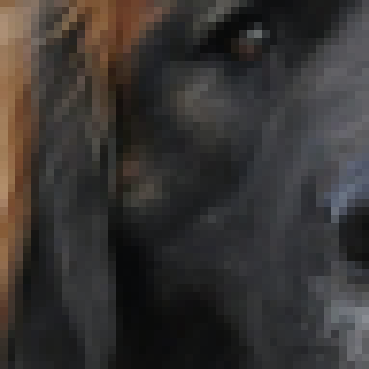}};

      \barplot[](\xTwo-0.035,\y-0.15)(0.03:0.02);
    \fi
    \ifnum\i=2 %
      \node[node in] (NO-\i) at (\xTwo,\y) {};

      \coordinate (c) at (\xTwo-0.65,\y);
      \draw[thick, colorSchemeTwo, fill=colorSchemeTwo!20,rounded corners=0.05cm] (c) \irregularcircle{0.65cm}{0.05cm};
      \node (rect) [blockTwo,xshift=0.0cm, yshift=-0.0cm] at (\xTwo-0.65,\y-0.15) {};
      \node[inner sep=0pt] (img) at (\xTwo-0.65,\y-0.15) {\includegraphics[width=0.5cm]{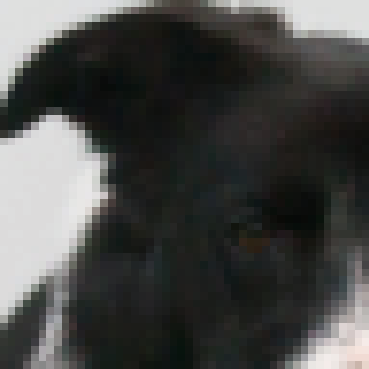}};
      \node (rect) [blockTwo,xshift=0.0cm, yshift=-0.0cm] at (\xTwo-0.75,\y+0.1) {};
      \node[inner sep=0pt] (img) at (\xTwo-0.75,\y+0.1) {\includegraphics[width=0.5cm]{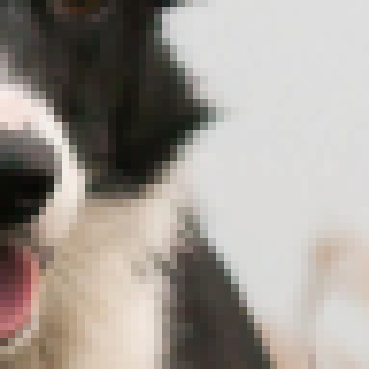}};
      \node (rect) [blockTwo,xshift=0.0cm, yshift=-0.0cm] at (\xTwo-0.55,\y+0.08) {};
      \node[inner sep=0pt] (img) at (\xTwo-0.55,\y+0.08) {\includegraphics[width=0.5cm]{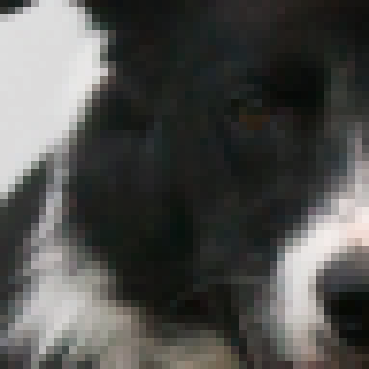}};
      \barplot[](\xTwo-0.035,\y-0.15)(0.26:0.16);
    \fi
    \ifnum\i=3 %
      \node[] (NO-\i) at (\xTwo,\y-0.35) {Bias};
      \node[node in] (NO-\i) at (\xTwo,\y) {};

      \barplot[](\xTwo-0.035,\y-0.15)(0.3:0.16);
    \fi
  }

  \foreach \i [evaluate={\c=int(\i==\NL); \y=\NL/2-\i-\c*\yshift; \index=(\i<\NL?int(\i):"m");}]
    in {\NO,...,1}{ %
        
    \ifnum\i=1 %
      \node[node in]
        (NL-\i) at (\xThree,\y) {}; %
      \barplot[](\xThree-0.035,\y-0.15)(0.28:0.29);
      \foreach \j [evaluate={\index=(\j<\NO?int(\j):"n");}] in {1,...,\NO}{ %
        \ifnum\j=1
            \draw[connect,white,line width=1.6] (NO-\j) -- (NL-\i);
            \draw[connect,line width=1.2] (NO-\j) -- (NL-\i)
              node[pos=0.87, black] {\contour{white}{-1}};
        \fi
        \ifnum\j=2
            \draw[connect,white,line width=1.2] (NO-\j) -- (NL-\i);
            \draw[connect] (NO-\j) -- (NL-\i)
              node[pos=0.75, black] {\contour{white}{0}};
        \fi
        \ifnum\j=3
            \draw[connect,white,line width=1.2] (NO-\j) -- (NL-\i);
            \draw[connect] (NO-\j) -- (NL-\i)
              node[pos=0.87, black] {\contour{white}{1}};
        \fi
      }
    \fi
  }

  \path (+0.4,0.1) node[colorSchemeOne] {$\hat{x}$};  
  \path (+0.4,-0.9) node[colorSchemeTwo] {$\tilde{x}$}; 
  
  \path (NO-\NO) --++ (0,4.35+\yshift-1.5) node[midway,scale=1.0] {$\vdots$};
  \path (NO-\NO) --++ (0+0.17,4.35+\yshift-1.5-0.25/2) node[midway,scale=1.0] {$m$};
  \path (NO-\NO) --++ (0+0.,0+2) node[scale=1.4, colorSchemeOne] {\contour{black!15}{$\hat{x}$}};

  \path (NO-\NO) --++ (0+0.,0+2) node[scale=1.4, colorSchemeOne] {\contour{black!15}{$\hat{x}$}};
  
  \path (NL-\NL) --++ (0+0.,0) node[scale=1.4, colorSchemeOne] {\contour{black!15}{$\neg \hat{x}$}};

\end{tikzpicture}
